# Supplementary material for: Simplicity in Auctions Revisited: The Primitive Complexity
Source: arXiv:2207.09853 source file (2022-07-20)
Supplement: Supplementary file 1 [file appendixold.tex]

\appendix

\subsection{A Linear Impossibility Result for Coverage Valuations \sd{move section to appendix}}
%As we show in Section~\ref{sec:algorithms}, for any sub-additive valuation, we can find an item of maximal value using polylogarithmic many queries.
%Before showing an exponential query complexity lower bound for the class of submodular valuation and general \opt{k} set, as a warm-up we start by showing that already for the class of coverage valuations, which is a subclass of submodular valuations, and the problem of finding a \opt{2} set, $\Om{n}$ demand queries are required. 
A valuation $v$ is a \emph{coverage} valuation if there exists a universe $U$ with non-negative weights $w(u)$ for each $u\in U$ and subsets $A_1, A_2,\ldots, A_n$ of $U$ such that $v(S) = \sum_{u\in \bigcup_{i\in S} A_i}w(u)$.

Consider the following coverage valuation over six items, $a,b1,b2,c1,c2,c3$, described in Figure~\ref{fig:cover}.
Formally, the universe $U = \set{x_{ijk}\mid (i,j)\in\set{(0,0),(0,1),(0,2),(1,1),(1,2)},~k\in\set{1,2,3}}$ has $15$ elements with weights $w(x_{1jk})=5,~w(x_{01k})=w(x_{02k})=3,~w(x_{00k})=7$ (see Figure~\ref{fig:cover}). The valuation $v$ is over $6$ items that correspond to the sets: $$a_1=\set{x_{1jk}},~b_1=\set{x_{i1k}},~b_2=\set{x_{i2k}},~c_1=\set{x_{ij1}},~c_2=\set{x_{ij2}},~c_3=\set{x_{ij3}}$$
for the above $i,j$ and $k$.
\comment{
$
v(a) = 30
v(b_i) = 24
v(c_j) = 23
v(a,bi) = 39
v(a,cj) = 
v(b1,b2) = 48
v(cj,ck) = 
b(bi,cj) =
v(a,bi,cj) = 
v(a,b1,b2) = 
v(a,cj,ck) = 
v(cj,b1,b2) = 
v(c1,c2,c3) = 69
v()
...
$
}
\begin{figure}
	\centering
	\includegraphics[width=0.7\linewidth]{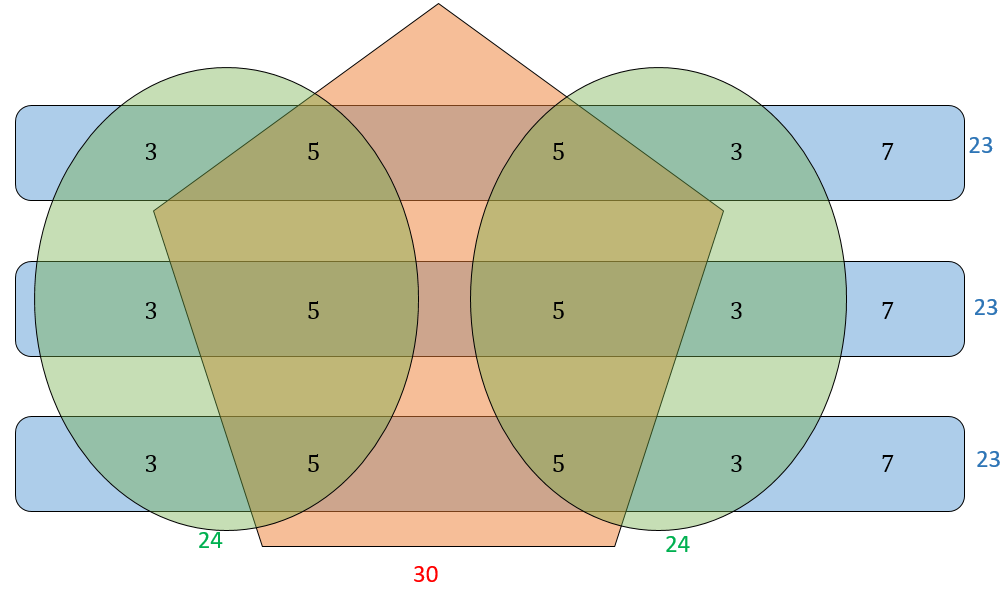}
	\caption{The 6-item coverage valuation. The 15 elements and weights are represented by the 15 black numbers, and each item is represented by a shape (the colored numbers demonstrates the values of the 6 singletons)}
	\label{fig:cover}
\end{figure}
We extend the 6-item valuation to a valuation over $m$ items by adding copies items for four of the items in the following way.
As before, the universe contains $15$ elements.
Each of the $m$ items corresponds to one of the six sets described above. We have a single copy of each of items $b_1$ and $b_2$, and $\frac{m-2}{4}$ copies of each of the other items.
Item $j$ is of {\em type} $A,C_1,C_2,C_3$ if it is a copy of $a,c_1,c_2,c_3$ respectively.
Let $\mathcal{F}$ be the family of valuations that are permutations of the above valuation, i.e., $v\in \mathcal{F}$ if there exists a re-naming of the items such that $v$ is identical to the described valuation up to the renaming. 

\begin{lemma}\label{lem:coverage_uniform}
	Consider a valuation $v\in\mathcal{F}$ and a uniform price query. The returned set never contains $b_1$ nor $b_2$.
\end{lemma}
\begin{proof}
	Fix some valuation $v\in\mathcal{F}$ and let $x$ be the uniform price for a single item.
	\begin{itemize}
		\item The profit from buying a single item is $30-x$ for any item of type $A$. 
		\item The profit from buying two items is bounded by $48-2x$. 
		\item The profit from buying three items is $69-3x$ for any $c_1,c_2,c_3$ items of types $C_1,C_2,C_3$ respectively.
	\end{itemize}
	For $x>18$ buying a single item of type $A$ dominates buying any other set of items. On the other hand, for $x<21$ buying three items from $C_1,C_2,C_3$ dominates buying any other set.  
\end{proof}

We now show that the fact that no uniform prices demand query returns a set of size $2$ implies that finding a maximal set of size $2$ requires learning the valuation of almost all sets of this size, thus resulting in a linear query complexity. 
\begin{theorem}
	Any algorithm that finds the bundle $S$, $|S|=2$, with the highest value in a coverage valuations and succeeds with constant probability, makes in expectation $\Omega(n)$ value and demand queries.
\end{theorem}
\begin{proof}
	Let $v$ be a valuation chosen from $\mathcal{F}$ uniformly at random. Observe that the optimal solution is to return the bundle that consists of $b_1$ and $b_2$. We claim by induction that in expectation, after making $r$ queries, for $r<n/500$ and $r>10$ \sd{but maybe we learn a lot from the first few queries?}, we learn the classification of at most $32r$ items of each type $A,C_1,C_2,C_3$, and thus cannot identify $b_1$ and $b_2$.
	%after $r$ queries (where $r<n/100\log n$), with probability $r\log n/ n$, it is impossible to identify the names of more than $r$ items from each of the non-best types.
	By the induction hypothesis, after $r$ queries there are at least $(n-2)/4-32r>n/8$ items from each type that their classification is unknown. \sd{so? how does this imply the theorem?}
	
	%Let $p_i$ be the price vector of the $r+1$ query.	
	Let $a,c_1,c_2,c_3$ be the cheapest items of types $A,C_1,C_2,C_3$ according to the $(r+1)$-th demand query, with prices $p_a,p_{c_1},p_{c_2},p_{c_3}$, respectively. Let $p_b$ be the minimum of the prices of $b_1$ and $b_2$.
	If $p_b\geq \max\set{p_a,p_{c_1},p_{c_2},p_{c_3}}$, by Lemma~\ref{lem:coverage_uniform} we are guaranteed that any set in the demand does not contain either $b_1$ or $b_2$ \sd{why? the lemma talks about uniform demand queries and no copies}.
	Since for each type at least $(m-2)/4-r>m/8$ of the items are indistinguishable \sd{what is indistinguishable?}, the probability that either one of $b_1$ and $b_2$ will be cheaper than all items of a certain type is upper bounded by $16/m$ and using the union bound, with probability at least 
	$1-\frac{64}{m}$, $b_1$ and $b_2$ are still unknown. If $b_1$ or $v_2$ are cheaper than all items of a certain type, we assume the algorithm succeeds in finding $b_1$ and $b_2$.
	
	We now claim that the information revealed \sd{what is "information revealed?"} by such a query is contained in the information revealed in the following process: The price vector in the $(r+1)$-th query defines an order over the items (with ties broken arbitrarily). We query the value of items by this order (with non-decreasing prices) one by one till we have one item from each type. Since at least $m/8$ of the unknown items are from the same type, after 8 such queries we are expected to sample from this type and after 32 samples we are expected to see all four types.
	
    Since there is no need of taking an item that is not the cheapest of its type, this information is enough in order to deduce the maximal profit. \sd{I don't understand this sentence}

	We have that in expectation, after $r+1$ queries there are at most $32(r+1)$ items that their type is known, and any pair selected by the algorithm as the returned set of size $2$ has a probability $o(m^{-2})$ to be the optimal one. \sd{why $m^{-2}$? what is the calculation?}
\end{proof}

\section{Missing Proofs} \label{app:missingproofs}
\subsection{Proof of Missing Lemmas for Theorem \ref{thm:findmaxkGS}}
We first prove the following general lemma (adjusted from \cite{leme2017gross}) regarding gross substitutes valuations.
\begin{lemma}\label{lem:S=T}
	Given a \GS{} function $f:2^{N}\rightarrow\mathbb{R}$ and two sets $S,T$ s.t. $|S|=|T|$ and any $s\in S\setminus T$, then $f(S)+f(T)\leq \max_{t\in T\setminus S}\left\lbrace f(S\setminus s\cup t)+f(T\setminus t\cup s)\right\rbrace.$
\end{lemma}
\begin{proof}
	For $|S \setminus T| = |T \setminus S| = 1$, the property in trivial.
	For $|S \setminus T| = |T \setminus S| = 2$, this follows directly from Lemma 4.3 in \cite{leme2017gross} \rk{cite formally}. 
	We now prove by induction on $k = |S \setminus T| = |T \setminus S|$.
	Fix some arbitrary $\tilde{s}\in (T \cup s)$ and find $\tilde{t}\in T\setminus S$	maximizing $f(T\cup\tilde{s}\setminus\tilde{t}) - f(S\cup\tilde{t}\setminus s)$.
	Now, apply induction on the sets $S$ and $T\cup \tilde{s}\setminus\tilde{t}$.
	We get that there is $t\in T\setminus(S\cup \tilde{t})$ such that:
	$$f(S)+f(T\cup\tilde{s}\setminus\tilde{t})\leq \max \set{f(S\cup t\setminus s)+f(T\cup\set{s,\tilde{s}}\setminus\set{t,\tilde{t}})}.$$
	By the case with $k = 2$ with sets $T$ and $T\cup\set{s,\tilde{s}}\setminus\set{t,\tilde{t}}$ we know that:
	$$f(T)+f(T\cup\set{s,\tilde{s}}\setminus\set{t,\tilde{t}})\leq \max \set{f(T\cup s\setminus t)+f(T\cup\tilde{s}\setminus\tilde{t}),f(T\cup\tilde{s}\setminus t)+f(T\cup s\setminus\tilde{t})}.$$
	If the maximum corresponds to the first expression, this together with the previous
	inequality, gives us exactly what we want to prove, i.e., $f(S)+f(T)\leq f(S\setminus s\cup t)+f(T\setminus t\cup s)$.
	If the maximum is the second expression we use the choice of $\tilde{t}$ to see that
	$f(T\cup\tilde{s}\setminus\tilde{t})-f(S\cup\tilde{t}\setminus s)\leq f(T\cup\tilde{s}\setminus t) - f(S\cup t\setminus s) $.
	This together with the previous inequalities also leads to the same result.
\end{proof}

We use the above Lemma to prove a version of matroid exchange property for gross substitutes valuations.
%\lemST*

\begin{proof}
	We define another function $f'$ on $n+|T|-|S|$ items by adding a set $D$ of size $|T|-|S|$ of dummy items: $f'(A \cup R) = f(A)$ for all $R\subseteq D$, i.e., adding $R$ does not affect the function value. It is straightforward to verify that $f'$ is a \GS{} function. Let $S' = S\cup D$, so $|S'|=|T|$. By Lemma~\ref{lem:S=T} over $f'$, $S',T$ and $s\in D\subseteq S'$, we get
	\[
	f(S)+f(T) = f'(S')+f'(T)\leq \max_{t\in T\setminus S'}\left\lbrace f'(S'\cup t\setminus s)+f'(T\cup s\setminus t)\right\rbrace = \max_{t\in T\setminus S}\left\lbrace f(S\cup t)+f(T\setminus t)\right\rbrace.\] 
\end{proof}

\subsection{Budget Additive}\label{app:BA}
%\thmfindmaxkBA*
\begin{proof}
	We first ask for the value $b$ of the grand bundle, which is the maximal value for any set $S\subseteq \items$ and a lower bound for the budget.
	Next, the algorithm samples a random item with non-zero value $t$. If it is known that all items have non-zero value, this is a trivial task. Otherwise, we find one using binary search: split the items randomly into two equal size sets and continue iteratively at random with any one of them who has value greater than zero.
	We make a demand for price $t/2$ for all items and receive a set $S$ of size $r$ and total value $v(S)=w$. If $r=k$, the algorithm found an optimal set. Else, there are several possible outcomes:
	\begin{itemize}
		\item $r < k$ and $w=b$.
		We can reach the maximal value $b$ by using the $r$ items of $S$ (and completing $S$ with any set of size $k-r$ since they all have a zero contribution).
		\item $r > k$ and $w<b$.
		We restrict the search to $S$, a subset of the items for which the valuation is additive (and thus solved using the algorithm from Theorem~\ref{thm:findmaxk}.
		\item $r < k$ and $w<b$. 
		We split our analysis: we first find an item of maximal value in $\items\setminus S$ (see Proposition~\ref{thm:findmaxSA}) and seeing if adding it reach $b$. If so, we have reached $b$ using at most $k$ items and we are done. Else, we have that $S$ contains all items of value at least $t$. This is since adding item of value $t\in \items\setminus S$ add marginal value $t$ (not capped by $b$) and cost $t$. Hence, in expectation, $S$ size is half of $\items$. We keep all items of $S$ and the algorithm continues on the remained set with $k=k-r$.
		\item $r > k$ and $w=b$.
		Observe that any set of size $r-1$ has a value strictly smaller than $b$ (since all prices are non-zero, all items have non-zero contribution), and the valuation is additive for any set of size $k$.
		We find best $k$ in $S$: choose an arbitrary item $a\in S$, and find the set $A$ of best $k$ in $S\setminus\set{a}$ (for which the valuation is additive), and find the minimal item $b\in A$ (that is, the gap between $A$ and the value of the best $k-1$ in $A$). We can replace $b$ in $a$ if indeed $a>b$ and thus we have found the best $k$ in $S$ (and we can find the minimal item in this set.
		Now, we make a demand for the price of the minimal item among the top $k$ in $S$ - the demand set has at least those $k$ items who are maximal in $S$. On the other hand, if it has $r$ items, we have that the marginal contribution of the least item is at least as much and the entire valuation on the returned set is additive and we are now back in case 2.
		% (removing one, solving, adding it. problem - many solutions of size $m$)
	\end{itemize}%
\end{proof}

\subsection{Finding the Largest Element}\label{app:SA}
%\thmfindmaxSA*
\mbc{maybe scope this in a proof environment}

In this section we prove that given a subadditive valuation $v$ over a set $\items$ of size $m$, there exists a randomized algorithm that finds an element of maximal value (a \opt{1} set) in $\O{\log^2 m}$ demand queries, in expectation.

The algorithm works as follows. Given a subadditive valuation $v$ over a set $\items$ of size $m$, the algorithm selects an item $j\in \items$ uniformly at random and sets $t=0$. 
%If $v(\items)=0$ it returns $j$. Otherwise it sets $t=0$  and 
It then runs the following iterative procedure:
\begin{itemize}
%     \item Run a uniform demand query with price $t$ for each item. Denote the set returned by the demand query by $T$. If $t\cdot |T|=v(T)$ then return item $j$ and terminate. 

	\item % If $T$ is empty or $v(T)= t\cdot|T| $ then, due to subadditivity, there is no item $k$ that has higher value than $t$. In this case the algorithm returns item $j$ and terminates. Else, we have that $v(T)>t\cdot|T|$, and the average value $t'={v(T)}/{|T|}$ is strictly larger than $t$. This implies, due to subadditivity, that there is at least one element of $T$ with value larger than $t$. 
	Let $L= \{ k\in \items| v({k})>t\}$ be the set of items such that each item has value strictly larger than $t$. 
	% As we have reached this step the set $L$ must be non-empty.  Now, by Lemma \ref{lem:random-larger},as $L$ is non-empty we can find a element from $L$ picked uniformly at random, in $O(\log m)$ demand queries in expectation. 	Let $i$ be the item returned. 
    We use Lemma \ref{lem:random-larger}
	to pick an element $i$ from $L$, uniformly at random, in $O(\log m)$ demand queries in expectation. 
    If no item was picked (the algorithm of the lemma terminated without returning an element), we return item $j$ and terminate. Otherwise,  
	we replace $j$ by $i$, set $t=v(\{i\})$, and reiterate (recomputing $L$ and so on). 
	\end{itemize}

    We first observe that the algorithm indeed returns an item of maximal value. % This is so as it keep the invariant that the sets $T$ and $L$ are never empty.  
    This is true as the value of $j$ monotonically increases and if the algorithm terminates and return $j$ it is because $L$ is empty, or equivalently, there is no other item has higher value (so $j$ is maximal). 
    %This is true for the first iteration as $v(\items)= 0$ implies that every item has value of $0$, so any item has maximal value (of zero).  After the first iteration we keep the invariant that in any iteration, any element of maximal value belongs to $L$, till the point in which an element of maximal value is returned and the algorithm terminates.

	We claim that within $O(\log m)$ iterations the algorithm terminates, as at each iteration the set of items of value above $t$ shrinks, in expectation, by factor of at least two (in expectation there are at least half the items that are smaller or equal to a random item value). As each iteration uses $O(\log m)$ demand queries in expectation, the algorithm uses $O(\log^2 m)$  demand queries in expectation. 

%	Given the lemma, the algorithm works in an iterative way, where at each round it eliminates, in expectation, at least half of the items (up to one), thus finishing after $\O{\log n}$ rounds, with each one having a logarithmic number of demand queries. 

\mbc{additive with ties in $O(\log^2 n)$  demand queries in expectation: 
use the lemma and claim this runs in log of the number of distinct values of singletons. 
}

===========================

In addition, we provide an example showing that for general (even monotone) valuations, $n-1$ demand queries are needed in order of finding an item of maximal value, even for randomized algorithms. 
\begin{example}\label{ex:genralvaluation}
	Consider the following family $\mathcal{F}=\{v_1,v_2,\ldots,v_n$ of $n$ valuations over $n$ items. 
	Valuation $v_i$ had item $i$ be of value $1$ (as a singleton), and each of the  other items has value $0$. 
	Any set of size $2$ or larger has a value of $2$.
\end{example}
\begin{proof}	
	Any demand query that prices two different items for a price smaller than (or equal to) $1$ for each of those items, returns the cheapest pair and reveals no information.
	On the other hand, if all prices are larger than $1$, the demand set is empty and again no information is revealed. 
	Thus, the only possibility of extracting information on the valuation, is by querying a single item for value smaller than $1$ (and all others strictly above) and a demand set reveals whether or not this is the item of value $1$.	
	Hence, $n-1$ queries are needed in order of finding the unique maximal item with probability larger than half, even with randomization (and any approximation for the maximal value).
\end{proof}

\section{The Main Algorithmic Result: Gross Substitutes Valuations}
\mbc{to be removed!}

\mbc{remark that greedy gives a polynomial upper bound (with value queries only)}

\mbc{move this to a different file and to the appendix for now. } 

In this section, we extend the pivotal idea beyond the algorithm for additive valuations and show algorithms for the two valuation classes of gross-substitutes and budget-additive. 

%We now continue with the class of budget-additive valuations.
%For this class, it is known that the welfare maximization problem cannot be solved for approximation better than $15/16$ using polynomial number of demand queries \rk{\citet{dughmi2015limitations} talk about it but I'm not sure who they are citing, and the lower bound might hold only for deterministic algorithms. or maybe im completely off}. Here we show that the cardinality maximization problem can be solved using polylogarithmic number of demand queries. 

The more \rk{interesting?general? economically motivated? rich? expressiveness?} is the class of gross-substitutes valuation. We extend our results for additive valuations and show an algorithm for gross-substitutes maximization with polylogarithmic query complexity.

\begin{theorem}\label{thm:findmaxkGS}
	Given a gross-substitutes valuation $v$ over a set $\items$ of size $m$, there exists a randomized algorithm that finds a \opt{k} set and has a query complexity of \rk{$polylog m$}.
\end{theorem}

An important characteristic of the class of gross-substitutes valuations is that any \opt{k} set can be achieved via the simple greedy algorithm that adds items of maximal marginal value as long as it is greater than zero, and that solutions are only different by the tie-breaking rule of the greedy algorithm (see \cite{leme2017gross}).
\begin{definition}
    Given a valuation $f$, the {\em greedy ordering} of $f$ over a set $\items$ of size $m$, with a tie-breaking rule $T$, is an ordering $a_1,a_2,\ldots,a_m$ of the items in $\items$ such that for any $i\in[m]$, we have that $a_i\in \arg\max_{x\in \items} f(x|\set{a_1,\ldots,a_{i-1}})$ and the choice of a specific item at each step is according to the tie breaking rule $T$.
\end{definition}

In our setting, Remark 5.5 from \cite{leme2017gross} can be stated as follow:
\begin{claim}\label{cla:greedy}(\cite{leme2017gross}, rephrased)
    Let $f$ a gross-substitutes valuation over $m$ items and $k\in [m]$.
    For any greedy ordering $a_1,a_2,\ldots,a_m$ of $f$, the prefix set $a_1,\ldots,a_k$ is a $\opt{k}$ set. Moreover, for any $\opt{k}$ set $S$, there exists a tie-breaking rule such that $S$ is a prefix of a greedy ordering of $f$.
\end{claim}

\rk{This greedy property guarantees that (up to ties), there exists a price $p$ such that a uniform demand query for this price returns a \opt{k} set (This is not true for general submodular valuations as we later show).
Unfortunately, this is not enough for the previous algorithm to work. Take for example the gross-substitutes valuation with $v(S) = |S|\cdot|S+1|/2$ for any set $S$ of items. For this valuation, the algorithm presented for additive valuations will take a linear number of demand queries regardless of the randomization. The key idea of the improved is that instead of using a random item's value as a pivot, we use a random marginal value by sampling a random set $R$ and a random item $j$ and setting $v(j|S)$ as our pivot.}

before describing the new algorithm, we show how to find efficiently a pair of maximal and minimal sizes sets in the demand for a given price vector. This assists us in handling ties, similarly to the approach taken in the additive case.

Since for any gross-substitutes valuation $v$ and price vector $p$, the valuation $f(S)=v(S)-p(S)$ is also a gross-substitutes valuation, an immediate corollary of claim~\ref{cla:greedy} is that any set in the demand for $p$ is a prefix of a greedy ordering of $f$ such that additional item will cause in a non-positive change in utility.
Hence, by looking at the corresponding ordering and removing all items of zero marginal value, we have that any set in the demand of maximal size contains a set in the demand of minimal size. We now describe an algorithm for finding such a pair.

\begin{lemma}\label{lem:getall}
	Let $v$ a gross-substitutes valuation over a set $\items$. Fix any subset of items $Z\subseteq \items$, a subset $\hat{Z}\subseteq Z$ and $j\in Z\setminus \hat{Z}$.
    Let $B$ be the prefix up to $j$ (exclusive) of some greedy ordering of $v$ over the set $\hat{Z}\cup\set{j}$. Suppose that $v(j|\hat{Z})>0$.
	Let $D'$ be a demand set when setting a uniform price  $p<v(j|\hat{Z})$ for every item $i\in Z$ (and infinity prices for every item $i\notin Z$).
	Then $|D'|>|B|$.
\end{lemma}
\begin{proof}
    Assume by contradiction that $|D'|<|B|+1 = |B\cup\set{j}|$. Then, by Lemma~\ref{lem:S>T}, there exist $t\in (B\cup\set{j})\setminus D'$ such that:
	\begin{equation*}
	v(D')+v(B\cup\set{j})\leq v(D'\cup\set{t})+v((B\cup\set{j})\setminus\set{t}) 
	\end{equation*}
	Rearranging:
	\begin{equation}\label{eq1gseq}
	v(B\cup\set{j}) - v((B\cup\set{j})\setminus\set{t})\leq v(D'\cup\set{t}) - v(D') 
	\end{equation}
	We now have that:
	\begin{eqnarray*}
		p& <    & v(\hat{Z}\cup\set{j}) - v(\hat{Z})\\
		& \leq & v(B\cup\set{j}) - v(B)\\
		& \leq & v(B\cup\set{j}) - v((B\cup\set{j})\setminus\set{t})\\
		& \leq & v(D'\cup\set{t}) - v(D').
	\end{eqnarray*}
	Where the first inequality is by the assumption $v(j|\hat{Z})>0$, the second by submodularity (as $B\subseteq \hat{Z}$), the third is since $B$ created using a greedy ordering of $\hat{Z}\cup\set{j}$ (and hence $v(B)>v((B\cup\set{j})\setminus\set{t})$) $|B|$ and the last by inequality \eqref{eq1gseq}.
	That is, $t$ can be added to $D'$ for price $p$ with positive utility in contradiction to $D'$ being in demand.
\end{proof}

\begin{lemma}\label{lem:getall}
	Given  a gross-substitutes valuation $v$ over a set $\items$ of size $m$, and a price vector $p$, there exists an algorithm with $\O{\log ^2 n}$ query complexity that finds two sets in the demand $D_{min}\subseteq D_{max}$, such that $|D_{max}|$ if maximal over all sets in the demand for price $p$ and $|D_{min}|$ is minimal over all such sets.
\end{lemma}
\begin{proof}
	The algorithm first makes a demand query for $p$. This splits the items into two sets, a set $D$ which is in the demand and $C=N\setminus D$.
    Without loss of generality, we can assume that $p$ is the all-zero price vector by embedding it within $v$ (since $v(S)-p(S)$ is also a gross-substitutes valuation). 
    
    %By Claim~\ref{cla:greedy}, there is a greedy ordering $a_1,\ldots,a_m$  that corresponds to $D$, i.e. $D = \set{a_1,\ldots,a_d}$ and $C = \set{a_{d+1},\ldots,a_m}$.
    %We wish to find a set $A = \set{a_i,\ldots,a_j}$ such that $D_{max} = D\cup A$ and $D_{min} = D\setminus A$.\footnote{Note that there might be several possible such sets. We abuse notation and denote by $A$ any such set.}

	We show how to find $D_{min}\subseteq D$. The algorithm for $D_{max}\supseteq D$ is similar \rk{and is detailed in appendix  XXX}. 
	
    The algorithm works in the following iterative way. Let $D_1$ be a random subset of $D$ of size $k$ (later to be defined), and $j$ a random item from $D\setminus D_1$.
	Assuming $v(j|D_1)>0$, the algorithm makes a demand query with uniform price $\frac{1}{2}v(j|D_1)$ for any item $i\in D$ (and infinity prices for items in $C$) and denote the returned set $D'$.\footnote{Without the assumption that $p$ is suppressed, the algorithm equivalently makes a query with price $p_i+v(j|D_1)/2$ for each item $i\in D$.} 
	
	We denote by $B$ the prefix up to $j$ (exclusive) of a greedy ordering (with random tie-breaking) of $v$ over the set $D_1\cup\set{j}$.
    %In addition, we denote by $G$ the prefix up to $j$ (exclusive) of the greedy ordering of $v(\cdot|R)$ over the set $(\items\setminus R)\cup\set{j}$. In both ordering we assume that ties are broken uniformly at random.
	We now show that $|D'|>|B|$. 
	Assume by contradiction that $|D'|<|B|+1 = |B\cup\set{j}|$. Then, by Lemma~\ref{lem:S>T}, there exist $t\in (B\cup\set{j})\setminus D'$ such that:
	\begin{equation*}
	v(D')+v(B\cup\set{j})\leq v(D'\cup\set{t})+v((B\cup\set{j})\setminus\set{t}) 
	\end{equation*}
	Rearranging:
	\begin{equation}\label{eq1gseq}
	v(B\cup\set{j}) - v((B\cup\set{j})\setminus\set{t})\leq v(D'\cup\set{t}) - v(D') 
	\end{equation}
	We now have that:
	\begin{eqnarray*}
		v(j|D_1)/2& <    & v(D_1\cup\set{j}) - v(D_1)\\
		& \leq & v(B\cup\set{j}) - v(B)\\
		& \leq & v(B\cup\set{j}) - v((B\cup\set{j})\setminus\set{t})\\
		& \leq & v(D'\cup\set{t}) - v(D').
	\end{eqnarray*}
	Where the first inequality is by the assumption $v(j|D_1)>0$, the second by submodularity (as $B\subseteq D_1$), the third is since $B$ created using a greedy ordering of $D_1\cup\set{j}$ (and hence $v(B)>v((B\cup\set{j})\setminus\set{t})$) $|B|$\mbc{unclear} and the last by inequality \eqref{eq1gseq}.
	That is, $t$ can be added to $D'$ for price $v(j|D_1)/2$ with positive utility in contradiction to $D'$ being in demand.
	We have that $\E{|B|} \geq k/2$ since $j$'s location is uniform \mbc{uniform at random?} among all items in $D_1\cup\set{j}$ and thus $\E{|D'|} \geq k/2$. 
	
	\mbc{need to formulate:} By guessing $k$ values ($(2^{-\ell})|D|$) we can find "the best" k to work with (i.e. a maximal one such that $v(j|D_1)$ is still larger than $0$ with good probability). 
	In expectation, after each iteration, $D\D'$ is getting smaller by a factor 2.
	repeating for log n iteration is good enough.

\mbc{Is the next a repeat of the above, or is there anything different?}

    The set $D_{max}$ is handled in similar way.
	The algorithm works in the following iterative way. Let $C_1$ be a random subset of $C$ of size $k$ (later to be defined), and $j$ a random item from $C\setminus C_1$.
	
	Assuming $v(j|D \cup C_1)<0$, the algorithm makes a demand query with uniform (negative) price $\frac{1}{2}v(j|D \cup C_1)$ for any item $i\in C$ (and zero prices for items in $D$) and denote the returned set $D'$. 
	
	we denote by $G$ the prefix up to $j$ (exclusive) of a greedy ordering (with random tie-breaking) of $v(\cdot|D\cup C_1)$ over the set $(C\setminus C_1)$.
	We now show that $|D'|\leq |D\cup C_1\cup G\leq \set{j}|$. 
	
	Assume by contradiction that $|D'|>|D \cup C_1\cup G\cup\set{j}|$. Then, by Lemma~\ref{lem:S>T}, there exist $t\in  D' \setminus (D \cup C_1\cup G\cup\set{j})$ such that:
	
	%Assume by contradiction that $|D'|>|D\cup C_1\cup G|$. Then, by Lemma~\ref{lem:S>T}, there exist $t\in  D' \setminus (D\cup C_1\cup G)$ such that:
	\begin{equation*}
	v(D')+v(D \cup C_1\cup G\cup\set{j})\leq v(D'\setminus\set{t})+v((D \cup C_1\cup G\cup\set{j})\cup\set{t}) 
	\end{equation*}
	Or:
	\begin{equation}\label{eq2gseq}
	v(D') - v(D'\setminus\set{t})\leq v((D \cup C_1\cup G\cup\set{j})\cup\set{t}) - v(D \cup C_1\cup G\cup\set{j})
	\end{equation}
	We now have that:
	\begin{eqnarray*}
		v(D') - v(D'\setminus\set{t})& \leq & v((D \cup C_1\cup G\cup\set{j})\cup\set{t}) - v(D \cup C_1\cup G\cup\set{j})\\
		& \leq & v((D \cup C_1\cup G\cup\set{j})\cup\set{t}) - v(D \cup C_1\cup G\cup\set{t})\\
		& \leq & v((D \cup C_1\cup\set{j}) - v(D \cup C_1) < \frac{1}{2}v(j|D \cup C_1)
	\end{eqnarray*}
	Where the first inequality is by inequality \eqref{eq2gseq}, the second is by the maximality of $R\cup G\cup\set{j}$ over sets of size $|R\cup G\cup\set{j}|$, third by submodularity, and the last is since $v(j|D \cup C_1)<0$.
	That is, $t$ can be added to $D'$ for price $v(j|D_1)/2$ with positive utility in contradiction to $D'$ being in demand.
	That is, $t$ can be removed from $D'$ getting back a price $\frac{1}{2}v(j|D \cup C_1)$ and positive utility, in contradiction to the fact that $D'$ is a set in the demand.
	
	We showed that $|D'|\leq |D\cup C_1\cup G|$. Hence, by the random selection of $j$ we have that $\E{|G|}\leq |D|+k+\frac{|C|-k}{2}$.

	By guessing $k$ values ($(1-2^{-i})|C|$)...
	Assuming $v(a|D \cup C_1)<0$ we are guaranteed that a maximal set of items of marginal zero is added (i.e., some possible set $A$).
	repeating for log n iteration is good enough.

\end{proof}

Next, we cite a Lemma from \cite{kupfer2020adaptive} (for completeness we give a full proof in Appendix~\ref{app:missingproofs}). Intuitively, the Lemma shows an augmentation property similar to the one we have for matroid valuations. 
%This property implies that not only an optimal set, \rk{?} %שניתן להשתמש בקבוצות מקריות יחסית כדי להרחיב פתרון אופטימלי קטן לפתרון אופטימלי גדול
\begin{lemma}\label{lem:S>T}(\cite{kupfer2020adaptive})
%\begin{restatable}[\cite{kupfer2020adaptive}]\label{lem:S>T}
	Given a gross-substitutes function $v$ and two sets $S,T$ s.t. $|S|<|T|$, then $v(S)+v(T)\leq \max_{t\in T\setminus S}\left\lbrace v(S\cup t)+v(T\setminus t)\right\rbrace.$
\end{lemma}

Using this lemma, we are now ready to present our proof for Theorem~\ref{thm:findmaxkGS}.

%\thmfindmaxkGS*
\begin{proof}
	The algorithm works in the following iterative way: at each round, we classify a fraction as the items as desired/undesired items, i.e., either returning a long prefix of the greedy algorithm or ruling out many items as being possibly selected (given the items already chosen).
	
	For each round round, let:
	\begin{itemize}
		\item $R$ - a random set of size $m/2$ chosen uniformly at random
		\item $j$ - an item chosen uniformly at random from $\items\setminus R$
		\item $p = v(R\cup\set{j}) - v(R)$ 
	\end{itemize}
	Next, using Lemma~\ref{lem:getall}, we find two sets in the demand $D_{max}$ and $D_{min}$ for uniform price $p$, such that $D_{min}\subseteq D_{max}$, $D_{max}$ if of maximal size and $D_{min}$ is of minimal size.
    We denote by $B$ the prefix up to $j$ (exclusive) of the greedy ordering of $v$ over the set $R\cup\set{j}$.
    In addition, we denote by $G$ the prefix up to $j$ (exclusive) of the greedy ordering of $v(\cdot|R)$ over the set $(\items\setminus R)\cup\set{j}$. In both ordering we assume that ties are broken uniformly at random.
	
	We first claim that $D_{max}$ is not too small by showing that $|D_{max}|>|B|$.
	
	Assume by contradiction that $|D_{max}|<|B\cup\set{j}|$. Then, by Lemma~\ref{lem:S>T}, there exist $t\in (B\cup\set{j})\setminus D_{max}$ such that:
	\begin{equation*}
	v(D_{max})+v(B\cup\set{j})\leq v(D_{max}\cup\set{t})+v((B\cup\set{j})\setminus\set{t}) 
	\end{equation*}
	Rearranging:
	\begin{equation}\label{eq1gs}
	v(B\cup\set{j}) - v((B\cup\set{j})\setminus\set{t})\leq v(D_{max}\cup\set{t}) - v(D_{max}) 
	\end{equation}
	We now have that:
	\begin{eqnarray*}
		p& =    & v(R\cup\set{j}) - v(R)\\
		& \leq & v(B\cup\set{j}) - v(B)\\
		& \leq & v(B\cup\set{j}) - v((B\cup\set{j})\setminus\set{t})\\
		& \leq & v(D_{max}\cup\set{t}) - v(D_{max}).
	\end{eqnarray*}
	Where the first inequality is by submodularity, the second is by the maximality of $B$ over sets of size $|B|$ contained in $R$ and the last by inequality \eqref{eq1gs}.
	That is, $t$ can be added to $D_{max}$ for price $p$ without harming the utility in contradiction to $D_{max}$ maximality.
	We have that $\E{|B|} = n/4$ since $j$'s location is symmetric among all items in $R\cup\set{j}$ and thus $\E{|D_{max}|} \geq n/4$.

	On the other direction, we similarly show that $D_{min}$ is not too large, namely $|D_{min}|\leq|R\cup G|+1$.	
	
	Assume by contradiction that $|D_{min}|>|R\cup G\cup\set{j}|$. Then, by Lemma~\ref{lem:S>T}, there exist $t\in  D_{min} \setminus (R\cup G\cup\set{j})$ such that:
	\begin{equation*}
	v(D_{min})+v(R\cup G\cup\set{j})\leq v(D_{min}\setminus\set{t})+v((R\cup G\cup\set{j})\cup\set{t}) 
	\end{equation*}
	Or:
	\begin{equation}\label{eq2gs}
	v(D_{min}) - v(D_{min}\setminus\set{t})\leq v((R\cup G\cup\set{j})\cup\set{t}) - v(R\cup G\cup\set{j})
	\end{equation}
	We now have that:
	\begin{eqnarray*}
		v(D_{min}) - v(D_{min}\setminus\set{t})& \leq & v((R\cup G\cup\set{j})\cup\set{t}) - v(R\cup G\cup\set{j})\\
		& \leq & v((R\cup G\cup\set{j})\cup\set{t}) - v(R\cup G\cup\set{t})\\
		& \leq & v((R\cup\set{j}) - v(R) = p
	\end{eqnarray*}
	Where the first inequality is by inequality \eqref{eq2gs}, the second is by the maximality of $R\cup G\cup\set{j}$ over sets of size $|R\cup G\cup\set{j}|$, and the last is by submodularity.
	That is, $t$ can be removed from $D_{min}$ without harming the total utility in contradiction to $D_{min}$ minimality.
	
	We have that $\E{|R\cup G|} = 3/4$  since $j$'s location is symmetric among all items in $R\cup\set{j}$ and thus $\E{|D_{min}|} < 3n/4$.
	
	By submodularity of gross-substitutes valuations, after getting $D_{min}$ and $D_{max}$ we can create a set $D$ such that $D$ is in the demand and $n/4\leq \E{|D_{min}|} \leq 3n/4$ by taking $D_{min}$ and adding any subset of $D_{max}\setminus D_{min}$. Next,
	\begin{itemize}
		\item If $|D|=k$, the algorithm found an optimal set of size $k$.
		\item If $|D|>k$, we know that there is an optimal set of size $k$ contained in $D$ and we can narrow our interest to a smaller item domain $D$ iteratively.
		\item If $|D|<k$, we know that $D$ is a prefix of a greedy algorithm and thus can be extended to an optimal set of size $k$. We keep all $D$ as a desired set and continue iteratively maximizing $v_{D}(\cdot)$ (which is also a gross-substitutes valuation) with the $k-|D|$ cardinality constraint
	\end{itemize}
	Since $\frac{n}{4}\leq \E{|D|}\leq \frac{3n}{4}$, the expected number of iterations is $\O{\log m}$.
\end{proof}
